# Supplementary material for: Anchor-based optimization of energy density functionals
Source: arXiv:2302.10979 source file (2023-03-22)
Supplement: Supplementary file 1 [file Supplemental-material.pdf]

# Supplemental material: Anchor-based optimization of energy density functionals

A. Taninah<sup>1</sup> and A. V. Afanasjev<sup>1</sup>

<sup>1</sup>*Department of Physics and Astronomy, Mississippi State University, MS 39762*

## I. OVERVIEW

Supplemental material provides additional information to the manuscript. The iterative procedure of the anchor based optimization method is discussed in Sec. II. Sec. III and Figs. 2 and 3 discuss the numerical errors due to truncation of the basis. The details of the fitting protocols and the input data to them are provided in Sec. IV and in Table IV. Tables V, VI and VII provide numerical values of the parameters of covariant energy density functionals (CEDFs) obtained in the present study. Finally, the calculated neutron skin thicknesses of the <sup>48</sup>Ca and <sup>208</sup>Pb are discussed in Sec. V.

## II. THE ITERATIVE PROCEDURE

The iterative procedure of anchor based optimization method is defined in the manuscript immediately after the introduction. Of particular interest is the behavior of the parameters  $\alpha_i$ ,  $\beta_i$  and  $\gamma_i$  of the correction function

$$E_{corr}(Z, N) = \alpha_i(N - Z) + \beta_i(N + Z) + \gamma_i \quad (1)$$

as a function of the counter  $i$  of the iteration. Their behavior is illustrated in Tables I, II and III on the examples of iterative procedures for the DD-MEX1, DD-MEY and NL5(Y) functionals. The iterative procedure is illustrated in Fig. 1 for the rms deviations  $\Delta E_{rms}$  between calculated and experimental binding energies  $E$  which represent the major contributor to the penalty function.

## III. NUMERICAL ACCURACY OF THE CALCULATIONS

The accuracy of numerical calculations depends on the truncation of the basis (see, for example, the detailed discussion in the appendix to Ref. [4]). In absolute majority of the DFTs calculations the question of whether the truncation of the basis under consideration provides an acceptable accuracy in the calculations of physical observables is defined by comparing the results of the calculations obtained with the  $N_F$  and  $N_F + 2$  fermionic shells. It is only in Ref. [5] an attempt was made to define the numerical errors of a given truncation of basis with respect of asymptotic limit at which the increase of basis does not change the results (see Sec. III in Ref. [5]).

Fig. 2 provides an example of such a comparison for the <sup>208</sup>Pb nucleus. One can see that binding energy curve comes close to the saturation at  $N_F \approx 26$ : above this

TABLE I. The values of the parameters  $\alpha_i$ ,  $\beta_i$  and  $\gamma_i$  of Eq. (1) of the paper defined at iteration  $i$  during the iterative procedure of the anchor based optimization method. The results are presented for iterative procedure of the DD-MEX1 functional and  $\Delta E_{rms}$  is global rms deviation of binding energies at  $i$ -th iteration.

| iteration<br>$i$ | $\Delta E_{rms}$<br>[MeV] | $\alpha_i$ | $\beta_i$ | $\gamma_i$ |
|------------------|---------------------------|------------|-----------|------------|
| 0                | 2.849                     | -0.075     | 0.0235    | -3.29      |
| 1                | 2.144                     | 0.044      | -0.028    | 2.55       |
| 2                | 2.139                     | -0.044     | 0.026     | -2.12      |
| 3                | 1.799                     | 0.165      | -0.070    | 4.95       |
| 4                | 2.607                     | -0.145     | 0.050     | -3.10      |
| 5                | 1.875                     | 0.055      | -0.025    | 2.05       |
| 6                | 1.826                     | -0.030     | 0.015     | -1.20      |
| 7                | 1.708                     | 0.020      | -0.010    | 0.80       |
| 8                | 1.651                     | -0.005     | 0.005     | -0.60      |
| 9                | 1.685                     | 0.020      | -0.010    | 0.75       |
| 10               | 1.713                     | 0.004      | -0.005    | -0.65      |
| 11               | 1.692                     | -0.009     | -0.002    | 0.29       |
| 12               | 1.646                     | -0.012     | 0.003     | 0.02       |
| 13               | 1.641                     | -0.010     | 0.002     | -0.01      |
| 14               | 1.637                     | -0.004     | 0.001     | 0.009      |

TABLE II. The same as Table I but for the DDMEY functional.

| iteration<br>$i$ | $\Delta E_{rms}$<br>[MeV] | $\alpha_i$ | $\beta_i$ | $\gamma_i$ |
|------------------|---------------------------|------------|-----------|------------|
| 0                | 2.589                     | 0.074      | -0.019    | -0.97      |
| 1                | 1.734                     | 0.003      | -0.001    | 0.10       |
| 2                | 1.739                     | 0.003      | 0.000     | -0.03      |
| 3                | 1.737                     | 0.002      | 0.000     | 0.01       |
| 4                | 1.738                     | -0.001     | 0.000     | 0.01       |

point the increase of  $N_F$  by two units changes the binding energy only by approximately 10 keV. Similar saturation properties have been seen for other functionals and for deformed nuclei. However, the numerical calculations are prohibitive at such sizes of the basis both because of the time of the calculations and the memory allocation problems. For example, the latter makes the deformed RHB calculations at available supercomputers impossible for  $N_F > 26$  without considerable changes in the code. At  $N_F < 20$ , the RHB calculations overbind the nuclei and the overbinding rapidly increases with the decrease of  $N_F$ .

Systematic global calculations of Ref. [2] and of the present paper as well as absolute majority of the CEDFs

TABLE III. The same as Table I but for the NL5(Y) functional.

| iteration<br>$i$ | $\Delta E_{rms}$<br>[MeV] | $\alpha_i$ | $\beta_i$ | $\gamma_i$ |
|------------------|---------------------------|------------|-----------|------------|
| 0                | 2.802                     | -0.108     | 0.030     | -1.80      |
| 1                | 2.362                     | 0.053      | -0.014    | 1.03       |
| 2                | 2.465                     | 0.043      | -0.005    | 0.64       |
| 3                | 2.360                     | 0.015      | -0.005    | 0.70       |
| 4                | 2.394                     | -0.021     | 0.000     | 0.25       |
| 5                | 2.384                     | -0.017     | 0.003     | -0.13      |
| 6                | 2.378                     | -0.012     | 0.003     | -0.08      |
| 7                | 2.378                     | -0.007     | 0.002     | -0.05      |
| 8                | 2.380                     | -0.001     | -0.001    | -0.04      |

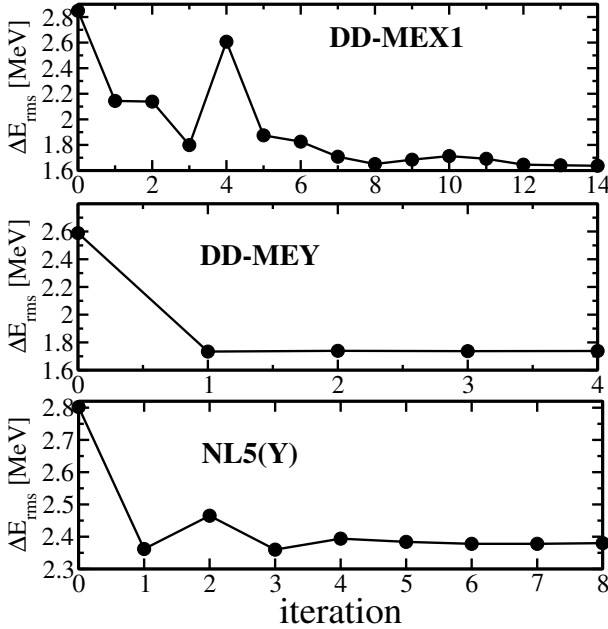

FIG. 1. The evolution of the rms deviations  $\Delta E_{rms}$  between calculated and experimental binding energies  $E$  as a function of iteration counter  $i$  in the anchor based optimization method for the indicated functionals.

fits (see, for example, Refs. [6–10]) are performed at  $N_F = 20$ . Fig. 2 shows that the binding energy calculated with  $N_F = 20$  deviates from asymptotic value of binding energy  $E(N_F \rightarrow \infty)$  by approximately 250 keV. This represents 0.015% error in the description of total binding energy. In reality, the errors of interest are substantially lower since the functionals are fitted to experimental binding energies [which are experimental analogs of  $E(N_F \rightarrow \infty)$ ] at  $N_F = 20$ . This means that substantial part of the difference between  $E(N_F = 20)$  and asymptotic value of binding energy  $E(N_F \rightarrow \infty)$  is accumulated in the parameters of the functional. Taking this fact into account it is important to carry out global calculations using the same truncation of basis as that used in the fitting protocol of the functional.

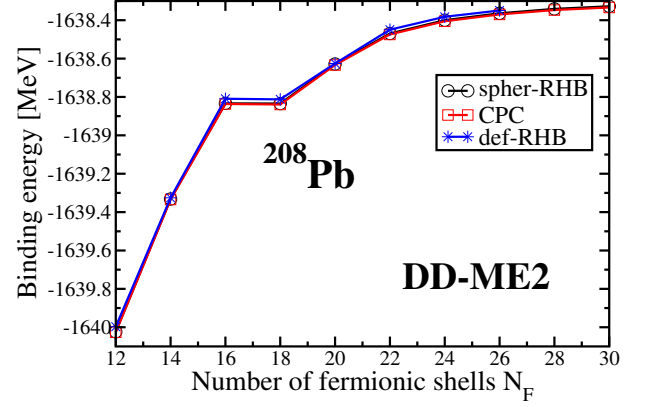

FIG. 2. The dependence of total binding energy of the  $^{208}\text{Pb}$  nucleus on the number of fermionic shells  $N_F$  for the DD-ME2 functional. The number of bosonic shells is fixed at  $N_B = 20$ . The calculations are performed with two spherical RHB codes: the one used in our group (labelled as "spher-RHB") and another which is published in Ref. [1] (labelled as "CPC"). These codes give exactly the same results. In addition, the results of the calculations with deformed RHB code (labelled as "def-RHB"), developed by us in Ref. [2], are shown. They slightly (by approximately 20 keV) differ from spherical results. This is most likely due to different arrangement of integration points in spherical and deformed calculations.

The reduction of the basis size in global calculations as compared with that used in the fitting protocol (as it is done in a number of studies) leads to numerical errors in the binding energies which are especially pronounced in heavy nuclei. This is illustrated in Fig. 3. One can see that numerical error given by  $E^{N_F=20} - E^{N_F=16}$  depends on employed functional and on the proton and neutron numbers. It is rather small for light nuclei but it increases in a complex way on going on to heavier nuclei. Let us consider the DD-MEX functional. For this functional, the  $E^{N_F=20} - E^{N_F=16}$  values range from 0 to 200 keV for the most of the nuclei with  $Z < 50$ , are located between 200 and 700 keV for the  $50 < Z < 102$  nuclei and reach the 700 – 900 keV range for the  $102 < Z < 122$  super-heavy nuclei [see Fig. 3(a)]. These observations confirm the view that, as  $Z$  and  $N$  increase, larger  $N_F$  is required to maintain the numerical accuracy of the description of binding energy. Similar general trend is seen in the results obtained with the PC-PK1 functional. However, there are some interesting differences between two functionals. Smaller basis leads to a larger binding for absolute majority of nuclei in the DD-ME2 functional. In contrast, there is a large area of the nuclear landscape shown in yellow in Fig. 3(b) in which the  $N_F = 16$  basis leads to a smaller binding as compared with the  $N_F = 20$  one.

TABLE IV. Input data for fitting protocols of the indicated CEDFs. The number  $n_i$  of experimental (empirical) data points and adopted errors  $\Delta O_{i,j}$  are presented for each type of data. N/A means that this type of data is not used in the fitting protocol. The references to already published functionals are provided.

|                                 | DD-ME2 [6]      | DD-MEX [7]      | DD-MEX1         | DD-MEX2        | DD-MEY         | NL5(E)         | NL5(Y)         | PC-PK1 [8] | PC-Y   | PC-Y1  |
|---------------------------------|-----------------|-----------------|-----------------|----------------|----------------|----------------|----------------|------------|--------|--------|
| 1                               | 2               | 3               | 4               | 5              | 6              | 7              | 8              | 9          | 10     | 11     |
| 1. Masses $E$ (MeV)             |                 |                 |                 |                |                |                |                |            |        |        |
| $n_1$                           | 12              | 12              | 12              | 12             | 12             | 12             | 12             | 60         | 60     | 12     |
| $\Delta E$ [MeV]                | $0.001E$        | $0.001E$        | $0.001E$        | 1.0            | 1.0            | $0.001E$       | 1.0            | 1.0        | 1.0    | 1.0    |
| 2. Charge radii $r_{ch}$ (fm)   |                 |                 |                 |                |                |                |                |            |        |        |
| $n_2$                           | 9               | 9               | 9               | 9              | 9              | 9              | 9              | 17         | 17     | 9      |
| $\Delta r_{ch}$ [fm]            | $0.002 r_{ch}$  | $0.002 r_{ch}$  | $0.002 r_{ch}$  | $0.002 r_{ch}$ | $0.002 r_{ch}$ | $0.002 r_{ch}$ | $0.002 r_{ch}$ | 0.02       | 0.02   | 0.02   |
| 3. Neutron skin $r_{skin}$ (fm) |                 |                 |                 |                |                |                |                |            |        |        |
| $n_3$                           | 3               | 3               | 3               | N/A            | N/A            | 4              | N/A            | N/A        | N/A    | N/A    |
| $\Delta r_{skin}$ [fm]          | $0.05 r_{skin}$ | $0.05 r_{skin}$ | $0.05 r_{skin}$ | N/A            | N/A            | exper. [9]     | N/A            | N/A        | N/A    | N/A    |
| 4. Nuclear matter properties    |                 |                 |                 |                |                |                |                |            |        |        |
| $n_4$                           | 4               | 4               | 4               | N/A            | N/A            | 4              | N/A            | N/A        | N/A    | N/A    |
| 5. Pairing interaction          |                 |                 |                 |                |                |                |                |            |        |        |
|                                 | Ref. [6]        | Pair-1          | Pair-1          | Pair-1         | Pair-2         | Pair-1         | Pair-2         | Ref. [8]   | Pair-2 | Pair-2 |

TABLE V. The parameters of the DDME CEDFs discussed in the present paper. The DD-ME2 and DD-MEX parameters are taken from Refs. [6, 7], respectively. The mass  $m$  of the nucleon is fixed at 939 MeV and the mass of  $\omega$ -meson at 783 MeV.

|                  | DD-ME2     | DD-MEX     | DD-MEX1    | DD-MEX2    | DD-MEY     |
|------------------|------------|------------|------------|------------|------------|
| $m_\sigma$ [MeV] | 550.123800 | 547.332728 | 553.714785 | 551.087886 | 551.321796 |
| $g_\sigma$       | 10.539600  | 10.706722  | 10.668226  | 10.476976  | 10.411867  |
| $g_\omega$       | 13.018900  | 13.338846  | 13.107751  | 12.903532  | 12.803298  |
| $g_\rho$         | 3.683600   | 3.619020   | 3.641508   | 4.100719   | 3.692170   |
| $b_s$            | 1.094300   | 1.334964   | 2.107233   | 1.506460   | 2.059712   |
| $c_s$            | 1.705700   | 2.067122   | 3.156692   | 2.337477   | 3.210289   |
| $c_o$            | 1.462000   | 1.605966   | 2.811153   | 2.100795   | 3.025356   |
| $a_r$            | 0.564700   | 0.620220   | 0.561222   | 0.193540   | 0.532267   |

TABLE VI. The parameters of the NLME CEDFs discussed in the present paper. The NL5(E) parameters are taken from Ref. [9]. The mass  $m$  of the nucleon is fixed at 939 MeV and the mass of  $\omega$ -meson at 782.6 MeV.

|                     | NL5(E)     | NL5(Y)     |
|---------------------|------------|------------|
| $m_\sigma$ [MeV]    | 503.298890 | 508.628825 |
| $g_\sigma$          | 10.263955  | 10.274835  |
| $g_\omega$          | 13.052487  | 12.906821  |
| $g_\rho$            | 4.582673   | 4.375307   |
| $g_2$ [fm $^{-1}$ ] | -10.976703 | -11.197664 |
| $g_3$               | -32.006687 | -31.996125 |

#### IV. FITTING PROTOCOLS

The optimization of the covariant energy density functionals to spherical nuclei in anchor-based optimization method is performed in the following way (see Ref. [9] for additional details). The objective function is defined for a model having  $N_{par}$  adjustable parameters  $\mathbf{p} = (p_1, p_2, \dots, p_{N_{par}})$  as

$$\chi^2(\mathbf{p}) = \sum_{i=1}^{N_{type}} \sum_{j=1}^{n_i} \left( \frac{O_{i,j}(\mathbf{p}) - O_{i,j}^{exp}}{\Delta O_{i,j}} \right)^2 \quad (2)$$

TABLE VII. The parameters of the PC CEDFs discussed in the present paper. The PC-PK1 parameters are taken from Ref. [8].

|                              | PC-PK1            | PC-Y              | PC-Y1             |
|------------------------------|-------------------|-------------------|-------------------|
| $\alpha_S$ [MeV $^{-2}$ ]    | $-0.396291^{-3}$  | $-0.405340^{-3}$  | $-0.394920^{-3}$  |
| $\alpha_V$ [MeV $^{-2}$ ]    | $0.269040^{-3}$   | $0.278770^{-3}$   | $0.268670^{-3}$   |
| $\alpha_{TV}$ [MeV $^{-2}$ ] | $0.295018^{-4}$   | $0.287940^{-4}$   | $0.293450^{-4}$   |
| $\beta_S$ [MeV $^{-5}$ ]     | $0.866530^{-10}$  | $0.837650^{-10}$  | $0.832870^{-10}$  |
| $\gamma_S$ [MeV $^{-8}$ ]    | $-0.380724^{-16}$ | $-0.375700^{-16}$ | $-0.344690^{-16}$ |
| $\gamma_V$ [MeV $^{-8}$ ]    | $-0.364219^{-17}$ | $-0.386340^{-17}$ | $-0.463780^{-17}$ |
| $\delta_S$ [MeV $^{-4}$ ]    | $-0.109108^{-9}$  | $-0.368410^{-9}$  | $-0.212860^{-9}$  |
| $\delta_V$ [MeV $^{-4}$ ]    | $-0.432619^{-9}$  | $-0.208240^{-9}$  | $-0.336750^{-9}$  |
| $\delta_{TV}$ [MeV $^{-4}$ ] | $0.411112^{-9}$   | $-0.557740^{-9}$  | $-0.470160^{-9}$  |

where number  $n_i$  is the number of experimental (empirical) data points of a given type and

$$N_{data} = \sum_{i=1}^{N_{type}} n_i \quad (3)$$

is the total number of data points of different types. Here,  $N_{type}$  stands for the number of different data types. The calculated and experimental/empirical values of physical observable  $j$  of the  $i$ -th type are represented by  $O_{i,j}(\mathbf{p})$  and  $O_{i,j}^{exp}$ , respectively.  $\Delta O_{i,j}$  is adopted error for physi-

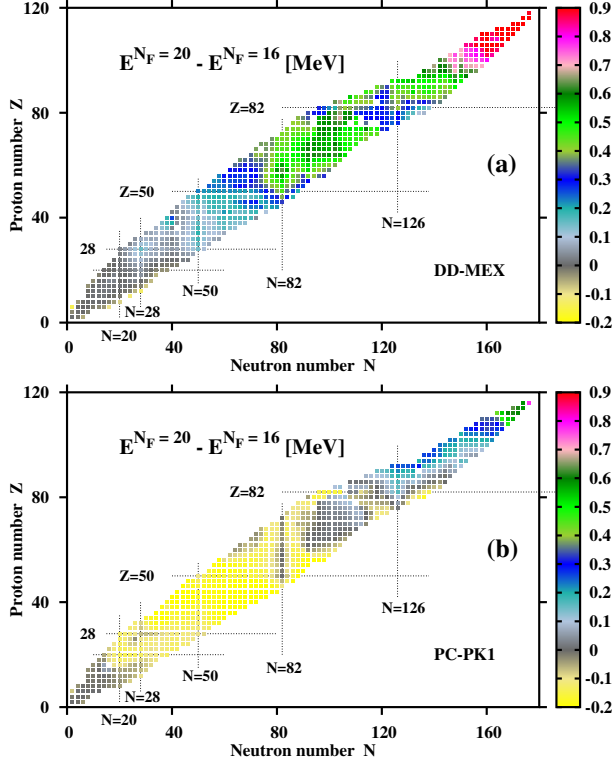

FIG. 3. The difference between the binding energies obtained in the global calculations with  $N_F = 16$  and  $N_F = 20$  for the DD-MEX and PC-PK1 functionals. The calculations include 855 even-even nuclei the binding energies of which are either measured or estimated in Ref. [3]. The nuclei in which the quadrupole deformations  $\beta_2$  of the ground states in these two calculations are significantly different ( $|\beta_2(N_F = 20) - \beta_2(N_F = 16)| > 0.05$ ) are excluded from consideration: they are shown by white squares.

cal observable  $O_{i,j}$ .

Table IV presents the details of the fitting protocols of CEDFs explored in the present paper. It includes the types of the data used in the fitting protocols and associated adopted errors. The nuclei and their experimental data used in these protocols are provided in Table 2 of Ref. [11] for the NLME and DDME functionals and in Tables II and III of Ref. [8] for the PC functionals. The distribution of 12 spherical anchor nuclei of Ref. [11] in nuclear chart is shown in Fig. 1(a) of Ref. [2]. Adopted errors for the nuclear matter properties of DDME and NL5(E) functionals follow Table 1 of the supplementary material of Ref. [7]. The parameters of the CEDFs for the DDME, NLME and PC classes of the functionals are summarized in Tables V, VI and VII, respectively.

## V. NEUTRON SKINS OF THE $^{48}\text{Ca}$ AND $^{208}\text{Pb}$ NUCLEI

An interesting issue is how the predicted neutron skin thicknesses  $r_{\text{skin}}$  compare with recent PREX-2 [12] and CREX [13] experiments. The values of  $r_{\text{skin}} = 0.283 \pm 0.071$  in  $^{208}\text{Pb}$  and  $r_{\text{skin}} = 0.121 \pm 0.026(\text{exp}) \pm 0.024(\text{model})$  in  $^{48}\text{Ca}$  have been defined in these experiments. To our knowledge this large difference of  $\Delta r_{\text{skin}} = r_{\text{skin}}(^{208}\text{Pb}) - r_{\text{skin}}(^{48}\text{Ca}) = 0.162$  fm (in the medium values of neutron skins) cannot be reproduced by any theoretical model [13–15], and existing and new CEDFs defined in this paper are not exception (see Table VIII). The large value of  $r_{\text{skin}}(^{208}\text{Pb})$  is best reproduced by the DD-MEX2, NL5(E), NL5(Y), PC-PK1, PC-Y and PC-Y1 functionals. They also produce the largest  $\Delta r_{\text{skin}}$  values ranging from  $\approx 0.06$  fm for NL5(\*) functionals to  $\approx 0.03$  fm for PC\* and DD-MEX2 functionals which, however, are substantially smaller than experimental value. The DD-ME2, DD-MEX, DD-MEX1 and DD-MEY functionals underestimate  $r_{\text{skin}}(^{208}\text{Pb})$  and provide quite small values for  $\Delta r_{\text{skin}} \approx 0.01$  fm. Note that the information on neutron skin thickness has been used only in fitting protocols of the DD-ME2, DD-MEX, DD-MEX1 and NL5(E) functionals (see Table IV). The analysis of the results presented in Table 1 of the paper suggests that the use of neutron skin thicknesses in the fitting protocols does not provide a reasonable constraint of the properties of CEDFs.

TABLE VIII. The neutron skins  $r_{\text{skin}}$  of the  $^{48}\text{Ca}$  and  $^{208}\text{Pb}$  nuclei for indicated functionals.

|            | $r_{\text{skin}}(^{48}\text{Ca})$<br>[fm] | $r_{\text{skin}}(^{208}\text{Pb})$<br>[fm] |
|------------|-------------------------------------------|--------------------------------------------|
| 1          | 2                                         | 3                                          |
| DD-ME2 [6] | 0.1868                                    | 0.1931                                     |
| DD-MEX [7] | 0.1838                                    | 0.1936                                     |
| DD-MEX1    | 0.1843                                    | 0.1952                                     |
| DD-MEX2    | 0.2265                                    | 0.2575                                     |
| DD-MEY     | 0.1897                                    | 0.1979                                     |
| NL5(E) [9] | 0.2288                                    | 0.2925                                     |
| NL5(Y)     | 0.2209                                    | 0.2759                                     |
| PC-PK1 [8] | 0.2320                                    | 0.2572                                     |
| PC-Y       | 0.2268                                    | 0.2598                                     |
| PC-Y1      | 0.2289                                    | 0.2567                                     |

[1] T. Nikšić, N. Paar, D. Vretenar, and P. Ring, Comp. Phys. Comm. **185**, 1808 (2014).

[2] S. E. Agbemava, A. V. Afanasjev, D. Ray, and P. Ring, Phys. Rev. C **89**, 054320 (2014).

- [3] M. Wang, G. Audi, F. G. Kondev, W. Huang, S. Naimi, and X. Xu, *Chinese Physics C* **41**, 030003 (2017).
- [4] A. V. Afanasjev, J. König, and P. Ring, *Nucl. Phys. A* **608**, 107 (1996).
- [5] S. E. Agbemava, A. V. Afanasjev, A. Taninah, and A. Gyawali, *Phys. Rev. C* **99**, 034316 (2019).
- [6] G. A. Lalazissis, T. Nikšić, D. Vretenar, and P. Ring, *Phys. Rev. C* **71**, 024312 (2005).
- [7] A. Taninah, S. E. Agbemava, A. V. Afanasjev, and P. Ring, *Phys. Lett. B* **800**, 135065 (2020).
- [8] P. W. Zhao, Z. P. Li, J. M. Yao, and J. Meng, *Phys. Rev. C* **82**, 054319 (2010).
- [9] S. E. Agbemava, A. V. Afanasjev, and A. Taninah, *Phys. Rev. C* **99**, 014318 (2019).
- [10] T. Nikšić, D. Vretenar, and P. Ring, *Phys. Rev. C* **78**, 034318 (2008).
- [11] G. A. Lalazissis, S. Karatzikos, R. Fossion, D. P. Arteaga, A. V. Afanasjev, and P. Ring, *Phys. Lett. B* **671**, 36 (2009).
- [12] D. Adhikari, H. Albatineh, D. Androic, K. Aniol, D. S. Armstrong, T. Averett, C. Ayerbe Gayoso, S. Barcus, V. Bellini, R. S. Beminiwattha, J. F. Benesch, H. Bhatt, D. Bhatta Pathak, D. Bhetuwal, B. Blaikie, Q. Campagna, A. Camsonne, G. D. Cates, Y. Chen, C. Clarke, J. C. Cornejo, S. Covrig Dusa, P. Datta, A. Deshpande, D. Dutta, C. Feldman, E. Fuchey, C. Gal, D. Gaskell, T. Gautam, M. Gericke, C. Ghosh, I. Halilovic, J.-O. Hansen, F. Hauenstein, W. Henry, C. J. Horowitz, C. Jantzi, S. Jian, S. Johnston, D. C. Jones, B. Karki, S. Katugampola, C. Keppel, P. M. King, D. E. King, M. Knauss, K. S. Kumar, T. Kutz, N. Lashley-Colthirst, G. Leverick, H. Liu, N. Liyange, S. Malace, R. Mammei, J. Mammei, M. McCaughan, D. McNulty, D. Meekins, C. Metts, R. Michaels, M. M. Mondal, J. Napolitano, A. Narayan, D. Nikolaev, M. N. H. Rashad, V. Owen, C. Palatchi, J. Pan, B. Pandey, S. Park, K. D. Paschke, M. Petrusky, M. L. Pitt, S. Premathilake, A. J. R. Puckett, B. Quinn, R. Radloff, S. Rahman, A. Rathnayake, B. T. Reed, P. E. Reimer, R. Richards, S. Riordan, Y. Roblin, S. Seeds, A. Shahinyan, P. Souder, L. Tang, M. Thiel, Y. Tian, G. M. Urciuoli, E. W. Wertz, B. Wojtsekhowski, B. Yale, T. Ye, A. Yoon, A. Zec, W. Zhang, J. Zhang, and X. Zheng (PREX Collaboration), *Phys. Rev. Lett.* **126**, 172502 (2021).
- [13] D. Adhikari, H. Albatineh, D. Androic, K. A. Aniol, D. S. Armstrong, T. Averett, C. Ayerbe Gayoso, S. K. Barcus, V. Bellini, R. S. Beminiwattha, J. F. Benesch, H. Bhatt, D. Bhatta Pathak, D. Bhetuwal, B. Blaikie, J. Boyd, Q. Campagna, A. Camsonne, G. D. Cates, Y. Chen, C. Clarke, J. C. Cornejo, S. Covrig Dusa, M. M. Dalton, P. Datta, A. Deshpande, D. Dutta, C. Feldman, E. Fuchey, C. Gal, D. Gaskell, T. Gautam, M. Gericke, C. Ghosh, I. Halilovic, J.-O. Hansen, O. Hassan, F. Hauenstein, W. Henry, C. J. Horowitz, C. Jantzi, S. Jian, S. Johnston, D. C. Jones, S. Kakkar, S. Katugampola, C. Keppel, P. M. King, D. E. King, K. S. Kumar, T. Kutz, N. Lashley-Colthirst, G. Leverick, H. Liu, N. Liyanage, J. Mammei, R. Mammei, M. McCaughan, D. McNulty, D. Meekins, C. Metts, R. Michaels, M. Mihovilovic, M. M. Mondal, J. Napolitano, A. Narayan, D. Nikolaev, V. Owen, C. Palatchi, J. Pan, B. Pandey, S. Park, K. D. Paschke, M. Petrusky, M. L. Pitt, S. Premathilake, B. Quinn, R. Radloff, S. Rahman, M. N. H. Rashad, A. Rathnayake, B. T. Reed, P. E. Reimer, R. Richards, S. Riordan, Y. R. Roblin, S. Seeds, A. Shahinyan, P. Souder, M. Thiel, Y. Tian, G. M. Urciuoli, E. W. Wertz, B. Wojtsekhowski, B. Yale, T. Ye, A. Yoon, W. Xiong, A. Zec, W. Zhang, J. Zhang, and X. Zheng (CREX Collaboration), *Phys. Rev. Lett.* **129**, 042501 (2022).
- [14] M. C. Atkinson, M. H. Mahzoon, M. A. Keim, B. A. Bodelon, C. D. Pruitt, R. J. Charity, and W. H. Dickhoff, *Phys. Rev. C* **101**, 044303 (2020).
- [15] B. Hu, W. Jiang, T. Miyagi, Z. Sun, A. Ekström, C. Forssén, G. Hagen, J. D. Holt, T. Papenbrock, S. R. Stroberg, and I. Vernon, nuclear theory archive arXiv:2112.01125v1 [nucl-th] **74**, 024312 (2022).
